# Supplementary material for: Learning Hamiltonian Dynamics with Reproducing Kernel Hilbert Spaces and Random Features
Source: arXiv:2404.07703 source file (2024-10-24)
Supplement: Supplementary file 1 [file Appendix.tex]

% \subsection{RFF for the curl-free kernel}

% The curl-free reproducing kernel $\boldK_c(\boldx,\boldz) = \boldG_c(\boldx-\boldz) \in \R^{n\times n}$ is derived the Gaussian kernel as \cite{Fuselier2006}
% \beq
%     \boldG_{c}(\boldx) = -\nabla \nabla^{\T}g_\sigma(\boldx) = \frac{1}{\sigma^2} e^{-\frac{\boldx^{\T} \boldx}{2 \sigma^2}} \left( \eye - \frac{\boldx \boldx^{\T}}{\sigma^2} \right)
% \eeq
% Differentiation of \eqref{eq_Bochner-gaussian} gives
% \begin{equation}\label{eq:Bochner_Gc}
%     \boldG_{c}(\boldx) = \inftyint \cos(\boldw^{\T}\boldx) \boldw \boldw^{\T} p_{\sigma}(\boldw) d\boldw
% \end{equation}
% It follows that
% \begin{equation}
%     \boldG_{c}(\boldx - \boldz) = \mbbE_{w}\bb \left(\cos(\boldw^{\T}\boldx)\cos(\boldw^{\T}\boldz) + \sin(\boldw^{\T}\boldx)\sin(\boldw^{\T}\boldz)\right) \boldw \boldw^{\T} \eb
% \end{equation}
% The matrix-valued curl-free kernel function can then be approximated by the matrix-valued feature map
% \begin{equation}
%     \boldPsi_{c}(\boldx) = \frac{1}{\sqrt{d}} 
%     \begin{bmatrix}
%         \cos(\boldw_{1}^{\T}\boldx)\boldw_{1}^{\T}\\
%         \vdots\\
%         \cos(\boldw_{d}^{\T}\boldx)\boldw_{d}^{\T}\\
%         \sin(\boldw_{1}^{\T}\boldx)\boldw_{1}^{\T}\\
%         \vdots\\
%         \sin(\boldw_{d}^{\T}\boldx)\boldw_{d}^{\T}
%     \end{bmatrix}
%     \in \R^{2d \times n}
% \end{equation}
% as
% \begin{equation}
%     \boldK_{c}(\boldx,\boldz) \approx \boldPsi_{c}(\boldx)^{\T} \boldPsi_{c}(\boldz)
% \end{equation}
% where $\boldw_i$ are drawn with distribution$p(\boldw)$. 
